# Supplementary material for: Scientific Information Extraction with Semi-supervised Neural Tagging
Source: arXiv:1708.06075 source file (2017-08-21)
Supplement: Supplementary file 1 [file Appendix.tex]

% \begin{table}[t]
%   \centering
%  {\small
%   \begin{tabular}{l|llll}
%     \toprule
%      Model & Overlap & Correct & False hit & Miss \\    
%     \midrule
%      SL & 568 & 1064 & 668 & 395\\
%      SSL & 533 & 1193 & 747 & 318\\
%     \bottomrule
%   \end{tabular}}
%   \caption{Error analysis on keyword identification task}
%   \label{tab:span}
% \end{table}

\begin{appendix}
\clearpage
\noindent{\huge\bfseries APPENDIX\par}
\section{Confusion Analysis}
\todo{not sure if needed or reformatted}
We then present the confusion matrix of SSL (our best system) as Fig.~\ref{fig:c_mat}

\begin{figure}[t]
\centering
\includegraphics[width=8cm]{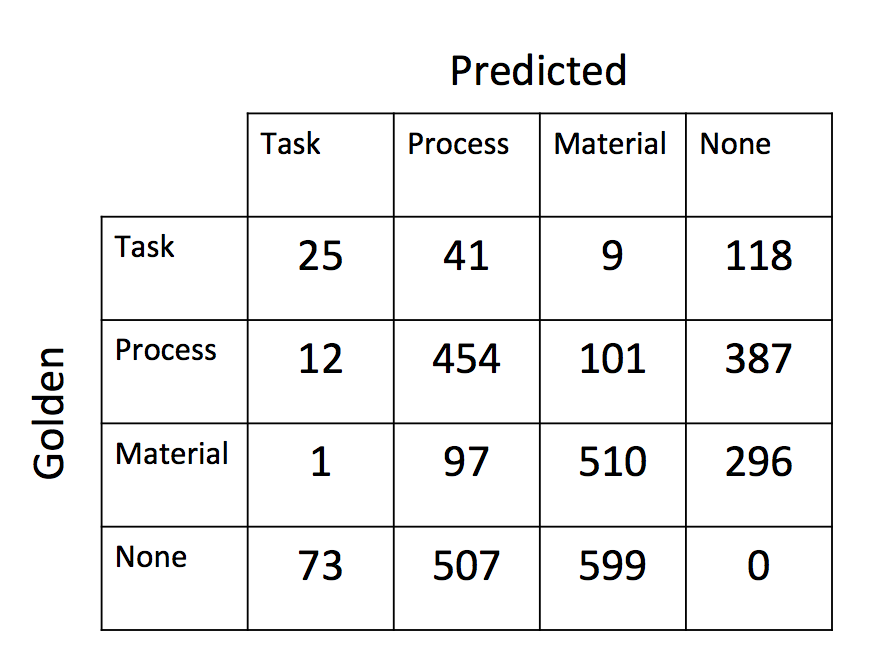}           
\caption{Confusion Matrix of SSL \todo{change to table}}
\label{fig:c_mat}
\end{figure}
\todo{percentage of multiple labels of a phrase: such as NER as task or method}
\end{appendix}
